# Supplementary material for: Statistical Mechanics of liquids and fluids in curved space
Source: arXiv:1005.2684 source file (2010-05-15)
Supplement: Supplementary file 1 [file PBC-Appendix.pdf]

# Periodic boundary conditions on the hyperbolic plane

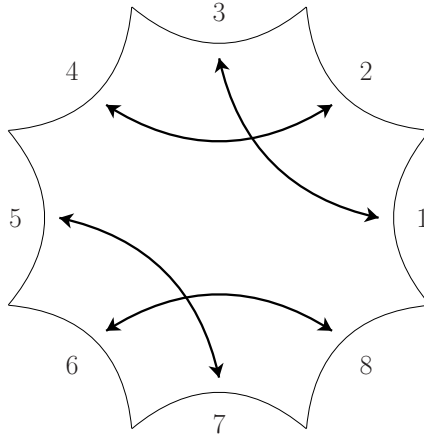

FIG. 1: Simplest fundamental polygon on the hyperbolic plane. It is associated to the  $\{8, 8\}$  tiling.

Generically, implementing periodic boundary conditions consists in choosing a primitive cell containing the physical system such that it can be infinitely replicated to tile the whole plane. So, prior to build periodic boundary conditions, one needs to know allowed tilings of the space considered. Here, for simplicity, we will limit ourself to regular cells and so to regular tilings.

On the hyperbolic plane, an infinity of regular tilings  $\{p, q\}$  are allowed if  $p$  (the number of edges of the primitive cell) and  $q$  (the number of cells meeting at each vertex of the tiling) verify the following condition

$$(p - 2)(q - 2) > 4. \quad (1)$$

It should lead to an infinity of possible periodic boundary conditions.

Let us go back to the general case. To ensure smoothness and consistency, the edges of the primitive cell of any periodic boundary condition have to be paired in a specific way: leaving the cell through one edge implies to come back by another edge, which should be equivalent to exploring the whole tiling of the plane. Constrains thus arise on how cell edges are paired together in addition to the shape of the cell. We will give in the following a rapid overview of how to classify and construct periodic boundary conditions on  $H^2$  by describing cell shapes and edge pairings. But before, let us describe the simplest case on the hyperbolic plane to introduce concepts needed to understand the classification.

First, a *fundamental polygon* (primitive cell with properly paired edges) encodes all the

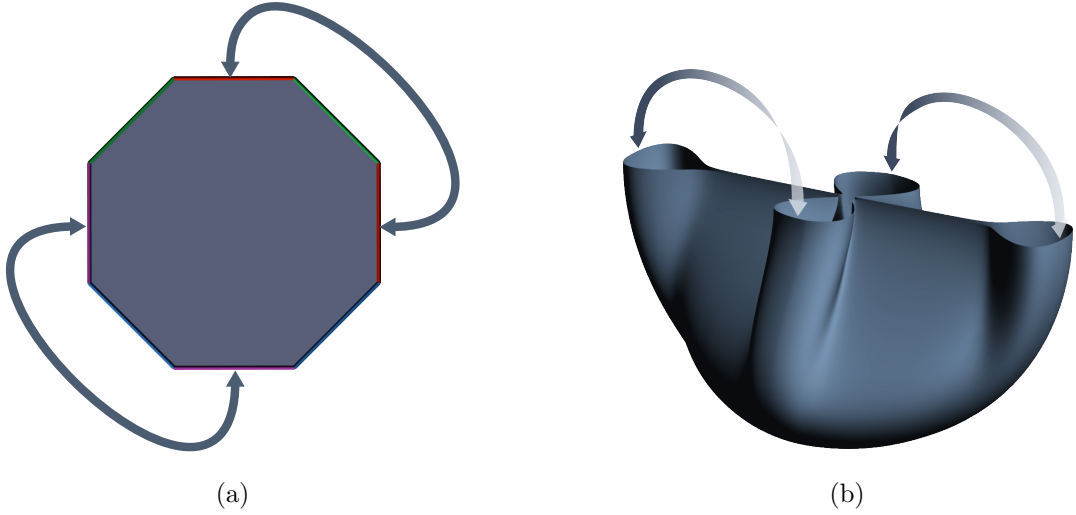

FIG. 2: Schematic representation of the “compactification” of the fundamental polygon shown in Fig. 1. The paired edges are glued together: 1 with 3 and 5 with 7 in (a); 2 with 4 and 6 with 8 in (b). The final compact manifold is a two-hole torus represented in Fig. 3.

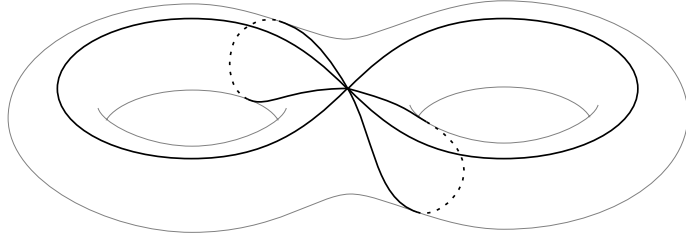

FIG. 3: Compact manifold and graph obtained by gluing the edges of the fundamental polygons of Fig. 1.

needed information to build periodic boundary conditions and to replicate the system on the entire space. The simplest (smallest) fundamental polygon on  $H^2$  is an octagon, corresponding to the  $\{8, 8\}$  tiling, whose pairing is shown in Fig. 1. By gluing the paired edges together (see Fig. 2 for of visualization of intermediate states) it is possible to represent the fundamental polygon as a compact manifold (see Fig. 3). It leads to a 2-hole torus, the genus (number of holes) of which is related to the area of the fundamental polygon through the Gauss-Bonnet theorem (cite?). As the genus is an integer, compact manifolds embedded in the hyperbolic plane can only access to a discrete subset of areas. In other words, homothety cannot be applied to hyperbolic manifolds without changing the curvature. Here,

the octagonal fundamental polygon cannot be scaled at constant curvature to allow to study a bigger system for instance. Thus, to change the area of the fundamental polygon in  $H^2$ , one has to vary its genus, which can be seen as adding/removing holes to the torus. Varying the genus of the polygon induces to change its symmetry, more particularly its number of edges.

To classify all the possibilities (for regular polygons), one can use the properties of the graph formed by glued edges of the fundamental polygon and embedded in the  $g$ -hole torus (see Fig. 3 for an example on the 2-hole torus). Constraints on such graphs to obtain relevant periodic boundary conditions are detailed in [?] and allow to classify and build all possible regular periodic boundary conditions in the hyperbolic plane [1]. The classification exhibits “families” based on the number of vertices of the graph embedded in the  $g$ -hole torus, which share similarities when varying  $g$ . In that framework, the octagonal fundamental polygon shown in Fig. 1 can be seen as the direct generalization of the square periodic boundary condition encountered in the Euclidean plane (both are in the same “family”).

To build periodic boundary conditions compatible with hyperbolic lattices to study spins systems for instance, a supplementary condition arises: the groups of symmetry of the fundamental polygon should be a special subgroup of the group associated to the lattice (see [?] for more details), which reduces the number of possible fundamental polygons. Thus the practical implementation of periodic boundary conditions is more complex for lattice systems than for continuous systems, which sounds unusual when compared to the usual Euclidean case.

---

[1] A tool to build such periodic boundary conditions can be found at the following address:

<http://physics.technion.ac.il/~sausset/CLP.html>
